# Supplementary material for: Final-state interactions in the CP asymmetries of charm-meson two-body decays
Source: arXiv:2305.11951 source file (2023-05-19)
Supplement: Supplementary file 1 [file old_appendices.tex]

\section{\toni{OLD: }Decay constants and form factors}
%%%\label{app:norm_sign_convs}
%\section{Normalization and sign conventions}

%is it strictly an effective theory including charm-mesons?/$m_c$ breaking is large
%expressions for $ \overline{D}^0 $: $ D^0 $ and $ \overline{D}^0 $ do not appear in the same process, so whatever extra sign you may get for $ \overline{D}^0 $ w.r.t. $ D^0 $ gets cancelled; see proceedings by Nierste

To fix conventions, we introduce the following pseudoscalar matrix \cite{Botella:1993va} %[we will not write down the mixing term of $ \pi^0 $ and $ \eta_8 $]

\begin{equation}\label{eq:U4_U4_chiral}
	\Pi = \begin{pmatrix}
		\frac{\eta_o}{2} {\color{black} +} \frac{\pi^0}{\sqrt{2}} + \frac{\eta_8}{\sqrt{6}} + \frac{\eta_{15}}{\sqrt{12}} & \pi^+ & K^+ & \overline{D}^0 \\
		\pi^- & \frac{\eta_o}{2} {\color{black} -} \frac{\pi^0}{\sqrt{2}} + \frac{\eta_8}{\sqrt{6}} + \frac{\eta_{15}}{\sqrt{12}} & K^0 & D^- \\
		K^- & \overline{K}^0 & \frac{\eta_o}{2} - \frac{2 \, \eta_8}{\sqrt{6}} + \frac{\eta_{15}}{\sqrt{12}} & D^-_S \\
		D^0 & D^+ & D^+_S & \frac{\eta_o}{2} - \frac{3 \, \eta_{15}}{\sqrt{12}} \\
	\end{pmatrix}
\end{equation}
{\color{red} In defining like so the charge-conjugation transformations of the mesons of interest are $C(\pi^+)=\pi^-, C(\pi^0)=\pi^0, C(K^+)=K^-, C(K^0)=\overline{K}^0$.}
The chiral Noether currents of the QCD Lagrangian ($v_\mu, a_\mu, s, p$ are external Hermitian matrix-valued fields)\footnote{We will later employ in App.~\ref{app:matrix_elements} factorization for four-fermion operators, so renormalizable interactions is all we discuss at this point.}
%[need to point out what happens in presence of four-quark operators from weak interactions]

\begin{eqnarray}
    && \mathcal{L}^0_{QCD} = - \frac{1}{4} G^a_{\mu \nu} G_a^{\mu \nu} + i \bar{q}_L \gamma^\mu D_\mu q_L + i \bar{q}_R \gamma^\mu D_\mu q_R \\
	&& \mathcal{L}_{QCD} = \mathcal{L}^0_{QCD} + \bar{q} \gamma^\mu ( v_\mu + \gamma_5 a_\mu ) q - \bar{q} ( s - i \gamma_5 p ) q
\end{eqnarray}
where

\begin{equation}
	r_\mu = v_\mu + a_\mu \,, \quad \ell_\mu = v_\mu - a_\mu
\end{equation}
and of the low-energy effective chiral Lagrangian with $ U = \text{exp} \left( i \sqrt{2} \Pi / F \right) $

\begin{equation}
	\mathcal{L}_2 = \frac{1}{4} F^2 \text{Tr} \left( D_\mu U^\dagger D^\mu U + U^\dagger \chi + \chi^\dagger U \right) \,, \quad \chi = 2 B_0 ( s + i p )
\end{equation}
are related as follows \cite{Pich:1995bw}

\begin{eqnarray}
	&& (J^\mu_L)^{ij} = \bar{q}_j \gamma^\mu P_L q_i = \frac{F}{\sqrt{2}} D^\mu \Pi^{ij} - \frac{1}{2} i \left( \Pi \, \overline{D^\mu} \, \Pi \right)^{ij} + \mathcal{O} (\Pi^3 / F) \\
	&& (J^\mu_R)^{ij} = \bar{q}_j \gamma^\mu P_R q_i = - \frac{F}{\sqrt{2}} D^\mu \Pi^{ij} - \frac{1}{2} i \left( \Pi \, \overline{D^\mu} \, \Pi \right)^{ij} + \mathcal{O} (\Pi^3 / F)
\end{eqnarray}
We will only keep the leading terms below. %[explain use of $\simeq$ (note e.g. $\mathcal{O} (\Pi^3 / F)$) and systematize it; I will keep only the leading terms]

Then %[$F_\pi, F_K$ are introduced in the next section] %[an overall sign from momentum everywhere has no physical effect]

\begin{eqnarray}
	&& \langle 0 | (J^\mu_A)^{12} | \pi^+ \rangle = \langle 0 | \bar{d} \gamma^\mu \gamma_5 u | \pi^+ \rangle = - \frac{2 F}{\sqrt{2}} (-i p^\mu) \\
	%
	&& \langle 0 | (J^\mu_A)^{21} | \pi^- \rangle = \langle 0 | \bar{u} \gamma^\mu \gamma_5 d | \pi^- \rangle = \langle 0 | (J^\mu_A)^{12} | \pi^+ \rangle \\
	%
	&& \langle 0 | (J^\mu_A)^{11} | \pi^0 \rangle = \langle 0 | \bar{u} \gamma^\mu \gamma_5 u | \pi^0 \rangle = \left( {\color{black} +} \frac{1}{\sqrt{2}} \right) \langle 0 | (J^\mu_A)^{12} | \pi^+ \rangle \\
	%
	&& \langle 0 | (J^\mu_A)^{22} | \pi^0 \rangle = \langle 0 | \bar{d} \gamma^\mu \gamma_5 d | \pi^0 \rangle = \left( {\color{black} -} \frac{1}{\sqrt{2}} \right) \langle 0 | (J^\mu_A)^{12} | \pi^+ \rangle
\end{eqnarray}
we then have

\begin{eqnarray}
	&& \langle 0 | \frac{( {\color{black} +} \bar{u} u {\color{black} -} \bar{d} d )_A}{\sqrt{2}} | \pi^0 (q) \rangle = \langle 0 | ( \bar{d} u )_A | \pi^+ (q) \rangle = \langle 0 | ( \bar{u} d )_A | \pi^- (q) \rangle \\
	&& \langle 0 | {\color{black} -} ( \bar{d} d )_A | \pi^0 (q) \rangle = \langle 0 | {\color{black} +} ( \bar{u} u )_A | \pi^0 (q) \rangle \\
    && \qquad = \frac{1}{\sqrt{2}} \langle 0 | ( \bar{d} u )_A | \pi^+ (q) \rangle = \frac{1}{\sqrt{2}} \langle 0 | ( \bar{u} d )_A | \pi^- (q) \rangle \nonumber
\end{eqnarray}
also

\begin{eqnarray}
	&& 2 \, m_d \langle 0 | {\color{black} -} ( \bar{d} d )_P | \pi^0 (q) \rangle = 2 \, m_u \langle 0 | {\color{black} +} ( \bar{u} u )_P | \pi^0 (q) \rangle \\
	&& \qquad = \frac{m_d + m_u}{\sqrt{2}} \langle 0 | ( \bar{d} u )_P | \pi^+ (q) \rangle = \frac{m_d + m_u}{\sqrt{2}} \langle 0 | ( \bar{u} d )_P | \pi^- (q) \rangle \nonumber
\end{eqnarray}

\begin{eqnarray}
	&& \langle 0 | (J^\mu_A)^{13} | K^+ \rangle = \langle 0 | \bar{s} \gamma^\mu \gamma_5 u | K^+ \rangle = - \frac{2 F}{\sqrt{2}} (-i p^\mu) \\
	%
	&& \langle 0 | (J^\mu_A)^{23} | K^0 \rangle = \langle 0 | \bar{s} \gamma^\mu \gamma_5 d | K^0 \rangle = \langle 0 | (J^\mu_A)^{13} | K^+ \rangle \\
	%
	&& \langle 0 | (J^\mu_A)^{31} | K^- \rangle = \langle 0 | \bar{u} \gamma^\mu \gamma_5 s | K^- \rangle = \langle 0 | (J^\mu_A)^{13} | K^+ \rangle \\
	%
	&& \langle 0 | (J^\mu_A)^{32} | \overline{K}^0 \rangle = \langle 0 | \bar{d} \gamma^\mu \gamma_5 s | \overline{K}^0 \rangle = \langle 0 | (J^\mu_A)^{13} | K^+ \rangle
\end{eqnarray}

\begin{eqnarray}
	&& {\color{black} +} \frac{1}{\sqrt{2}} \times \langle \pi^+ | (J^\mu_V)^{41} | D^+ \rangle = {\color{black} +} \frac{1}{\sqrt{2}} \times \langle \pi^+ | \bar{u} \gamma^\mu c | D^+ \rangle \\
    && \qquad = \langle \pi^0 | (J^\mu_V)^{41} | D^0 \rangle = \langle \pi^0 | \bar{u} \gamma^\mu c | D^0 \rangle \nonumber \\
	%
	&& \langle \pi^0 | (J^\mu_V)^{42} | D^+ \rangle = \langle \pi^0 | \bar{d} \gamma^\mu c | D^+ \rangle \\
    && \qquad = {\color{black} -}\frac{1}{\sqrt{2}} \times \langle \pi^- | (J^\mu_V)^{42} | D^0 \rangle = {\color{black} -}\frac{1}{\sqrt{2}} \times \langle \pi^- | \bar{d} \gamma^\mu c | D^0 \rangle \nonumber \\
	%
	&& \langle \overline{K}^0 | (J^\mu_V)^{43} | D^+ \rangle = \langle \overline{K}^0 | \bar{s} \gamma^\mu c | D^+ \rangle = \langle K^- | (J^\mu_V)^{43} | D^0 \rangle = \langle K^- | \bar{s} \gamma^\mu c | D^0 \rangle
	%
\end{eqnarray}

We also have

\begin{eqnarray}
	&& \langle \pi^0 | ( \bar{u} c )_V | D^0 \rangle = {\color{black} +} \frac{1}{\sqrt{2}} \langle \pi^- | ( \bar{d} c )_V | D^0 \rangle \,, \\
    && (m_c-m_u) \langle \pi^0 | ( \bar{u} c )_S | D^0 \rangle = {\color{black} +} (m_c-m_d) \frac{1}{\sqrt{2}} \langle \pi^- | ( \bar{d} c )_S | D^0 \rangle
\end{eqnarray}

%\begin{equation}
%	\langle \pi^0 | ( \bar{d} c )_V | D^+ \rangle = {\color{red} -}\frac{1}{\sqrt{2}} \langle \pi^- | ( \bar{d} c )_V | D^0 \rangle \,, \quad \langle \overline{K}^0 | ( \bar{s} c )_V | D^+ \rangle = \langle K^- | ( \bar{s} c )_V | D^0 \rangle
%\end{equation}

\section{\toni{OLD:} Factorization of matrix elements}\label{app:matrix_elements}
%\section{Predictions based on large-$ N_c $; form-factors and decay constants}

%Branco et al.: ``The precision of this method is limited by the $SU(3)$-breaking effects. Although $ f_K / f_\pi $ should be the dominant $SU(3)$ breaking correction, and factorization provides a reasonable approximation for the matrix elements of the current-current operators, factorization of the matrix elements of penguin operators is questionable.''

%[\textbf{TODO:} mostly done]

Each operator in Eq.~\eqref{eq:H_eff} contributes with a tree topology with different spectator quarks; $ \langle Q_{3,5} \rangle_{tree} $ do not contribute, as $ \langle \pi^0 | ( \bar{u} u {\color{black} +} \bar{d} d )_A | 0 \rangle = 0 $.
Annihilation topology gives contributions proportional to $ M_{P_1} - M_{P_2} $ for final states $ P_1 P_2 = \pi^+ \pi^- $, $ \pi^0 \pi^0 $, $ K^+ K^- $, $ K^0 \overline{K}^0 $, $ \pi^+ \pi^0 $, $ K^+ \overline{K}^0 $.
Exchange topology gives contributions suppressed by large $ N_C $; the same for gluonic dipole insertions.
%I will not say "long-distance penguin as well", it could be interpreted wrongly
%We omit at times the final state below:
The relevant matrix elements are the following ones:

%%%%%%%%%%%%%%%%%%%%%%%%%%%%%%%

\begin{equation}
	\langle Q_1^d \rangle_{tree; \pi^+ \pi^-} = \langle ( \bar{d} c )_{V-A} ( \bar{u} d )_{V-A} \rangle_{tree} = \langle \pi^- | ( \bar{d} c )_{V-A} | D^0 \rangle \langle \pi^+ | ( \bar{u} d )_{V-A} | 0 \rangle \\
	%&& \langle Q_1^d \rangle_{tree} = \langle ( \bar{d} c )_{V-A} ( \bar{u} d )_{V-A} \rangle_{tree} = \langle \pi^0 | ( \bar{d} c )_{V-A} | D^+ \rangle \langle \pi^+ | ( \bar{u} d )_{V-A} | 0 \rangle \nonumber
\end{equation}

\begin{equation}
	\langle Q_1^d \rangle_{tree; \pi^+ \pi^0} = {\color{black} -}\frac{1}{\sqrt{2}} \langle \pi^- | ( \bar{d} c )_{V-A} | D^0 \rangle \langle \pi^+ | ( \bar{u} d )_{V-A} | 0 \rangle
\end{equation}

%%%%

\begin{equation}
	\langle Q_2^d \rangle_{tree; \pi^0 \pi^0} = \langle ( \bar{u} c )_{V-A} ( \bar{d} d )_{V-A} \rangle_{tree} = {2 \times} \langle \pi^0 | ( \bar{u} c )_{V-A} | D^0 \rangle \langle \pi^0 | ( \bar{d} d )_{V-A} | 0 \rangle \label{eq:eq_Q2d}\\
	%&& \langle Q_2^d \rangle_{tree} = \langle ( \bar{u} c )_{V-A} ( \bar{d} d )_{V-A} \rangle_{tree} = \langle \pi^+ | ( \bar{u} c )_{V-A} | D^+ \rangle \langle \pi^0 | ( \bar{d} d )_{V-A} | 0 \rangle \nonumber
\end{equation}

\begin{equation}
	\langle Q_2^d \rangle_{tree; \pi^+ \pi^0} = {\color{black} +} \sqrt{2} \langle \pi^0 | ( \bar{u} c )_{V-A} | D^0 \rangle \langle \pi^0 | ( \bar{d} d )_{V-A} | 0 \rangle
\end{equation}

%%%%

\begin{equation}
	\langle Q_1^s \rangle_{tree; K^+ K^-} = \langle ( \bar{s} c )_{V-A} ( \bar{u} s )_{V-A} \rangle_{tree} = \langle K^- | ( \bar{s} c )_{V-A} | D^0 \rangle \langle K^+ | ( \bar{u} s )_{V-A} | 0 \rangle \\
	%&& \langle Q_1^s \rangle_{tree} = \langle ( \bar{s} c )_{V-A} ( \bar{u} s )_{V-A} \rangle_{tree} = \langle \overline{K}^0 | ( \bar{s} c )_{V-A} | D^+ \rangle \langle K^+ | ( \bar{u} s )_{V-A} | 0 \rangle \nonumber
\end{equation}

\begin{equation}
	\langle Q_1^s \rangle_{tree; K^+ \overline{K}^0} = \langle K^- | ( \bar{s} c )_{V-A} | D^0 \rangle \langle K^+ | ( \bar{u} s )_{V-A} | 0 \rangle
\end{equation}

%%%%
%the sum runs for u, d

%\begin{eqnarray}
%	&& \langle Q_3 \rangle_{tree} = \langle ( \bar{u} c )_{V-A} \Sigma_q ( \bar{q} q )_{V-A} \rangle_{tree} = \langle \pi^0 | ( \bar{u} c )_{V-A} | D^0 \rangle \langle \pi^0 | ( \bar{u} u + \bar{d} d )_{V-A} | 0 \rangle \\
%	&& \langle Q_3 \rangle_{tree} = \langle ( \bar{u} c )_{V-A} \Sigma_q ( \bar{q} q )_{V-A} \rangle_{tree} = \langle \pi^+ | ( \bar{u} c )_{V-A} | D^+ \rangle \langle \pi^0 | ( \bar{u} u + \bar{d} d )_{V-A} | 0 \rangle \nonumber
%\end{eqnarray}

%%%%
%the sum runs for u, d, s

\begin{equation}
	\langle Q_4 \rangle_{tree; \pi^+ \pi^-} = \langle \Sigma_q ( \bar{q} c )_{V-A} ( \bar{u} q )_{V-A} \rangle_{tree} = \langle \pi^- | ( \bar{d} c )_{V-A} | D^0 \rangle \langle \pi^+ | ( \bar{u} d )_{V-A} | 0 \rangle = \langle Q_1^d \rangle_{tree}
	%&& \langle Q_4 \rangle_{tree} = \langle \Sigma_q ( \bar{q} c )_{V-A} ( \bar{u} q )_{V-A} \rangle_{tree} = \langle \pi^0 | ( \bar{d} c )_{V-A} | D^+ \rangle \langle \pi^+ | ( \bar{u} d )_{V-A} | 0 \rangle \nonumber
\end{equation}

\begin{equation}
	\langle Q_4 \rangle_{tree; \pi^+ \pi^0} = {\color{black} -}\frac{1}{\sqrt{2}} \langle \pi^- | ( \bar{d} c )_{V-A} | D^0 \rangle \langle \pi^+ | ( \bar{u} d )_{V-A} | 0 \rangle
\end{equation}

%%%%

\begin{equation}
	\langle Q_4 \rangle_{tree; K^+ K^-} = \langle K^- | ( \bar{s} c )_{V-A} | D^0 \rangle \langle K^+ | ( \bar{u} s )_{V-A} | 0 \rangle = \langle Q_1^s \rangle_{tree}
	%&& \langle Q_4 \rangle_{tree} = \langle \overline{K}^0 | ( \bar{s} c )_{V-A} | D^+ \rangle \langle K^+ | ( \bar{u} s )_{V-A} | 0 \rangle \nonumber
\end{equation}

\begin{equation}
	\langle Q_4 \rangle_{tree; K^+ \overline{K}^0} = \langle K^- | ( \bar{s} c )_{V-A} | D^0 \rangle \langle K^+ | ( \bar{u} s )_{V-A} | 0 \rangle
\end{equation}

%%%%

\begin{equation}
	\langle Q_4 \rangle_{tree; \pi^0 \pi^0} = {2 \times} \langle \pi^0 | ( \bar{u} c )_{V-A} | D^0 \rangle \langle \pi^0 | ( \bar{u} u )_{V-A} | 0 \rangle = {\color{black} -} \langle Q_2^d \rangle_{tree} \label{eq:eq_Q4}
	%&& \langle Q_4 \rangle_{tree} = \langle \pi^+ | ( \bar{u} c )_{V-A} | D^+ \rangle \langle \pi^0 | ( \bar{u} u )_{V-A} | 0 \rangle \nonumber
\end{equation}

\begin{equation}
	\langle Q_4 \rangle_{tree; \pi^+ \pi^0} = {\color{black} +} \sqrt{2} \langle \pi^0 | ( \bar{u} c )_{V-A} | D^0 \rangle \langle \pi^0 | ( \bar{u} u )_{V-A} | 0 \rangle
\end{equation}

%%%%
%the sum runs for u, d, s

%\begin{eqnarray}
%	&& \langle Q_5 \rangle_{tree} = \langle ( \bar{u} c )_{V-A} \Sigma_q ( \bar{q} q )_{V+A} \rangle_{tree} = \langle \pi^0 | ( \bar{u} c )_{V-A} | D^0 \rangle \langle \pi^0 | ( \bar{u} u + \bar{d} d )_{V+A} | 0 \rangle \\
%	&& \langle Q_5 \rangle_{tree} = \langle ( \bar{u} c )_{V-A} \Sigma_q ( \bar{q} q )_{V+A} \rangle_{tree} = \langle \pi^+ | ( \bar{u} c )_{V-A} | D^+ \rangle \langle \pi^0 | ( \bar{u} u + \bar{d} d )_{V+A} | 0 \rangle \nonumber
%\end{eqnarray}

%%%%
%the sum runs for u, d, s

\begin{equation}
	\langle Q_6 \rangle_{tree; \pi^+ \pi^-} = -2 \, \langle \Sigma_q ( \bar{q} c )_{S-P} ( \bar{u} q )_{S+P} \rangle_{tree} = -2 \, \langle \pi^- | ( \bar{d} c )_{S-P} | D^0 \rangle \langle \pi^+ | ( \bar{u} d )_{S+P} | 0 \rangle \\
	%&& \langle Q_6 \rangle_{tree} = -2 \, \langle \Sigma_q ( \bar{q} c )_{S-P} ( \bar{u} q )_{S+P} \rangle_{tree} = -2 \, \langle \pi^0 | ( \bar{d} c )_{S-P} | D^+ \rangle \langle \pi^+ | ( \bar{u} d )_{S+P} | 0 \rangle \nonumber
\end{equation}

\begin{equation}
	\langle Q_6 \rangle_{tree; \pi^+ \pi^0} = {\color{black} +}2 \, \frac{1}{\sqrt{2}} \langle \pi^- | ( \bar{d} c )_{S-P} | D^0 \rangle \langle \pi^+ | ( \bar{u} d )_{S+P} | 0 \rangle
\end{equation}

%%%%

\begin{equation}
	\langle Q_6 \rangle_{tree; K^+ K^-} = -2 \, \langle K^- | ( \bar{s} c )_{S-P} | D^0 \rangle \langle K^+ | ( \bar{u} s )_{S+P} | 0 \rangle \\
	%&& \langle Q_6 \rangle_{tree} = -2 \, \langle \overline{K}^0 | ( \bar{s} c )_{S-P} | D^+ \rangle \langle K^+ | ( \bar{u} s )_{S+P} | 0 \rangle \nonumber
\end{equation}

\begin{equation}
	\langle Q_6 \rangle_{tree; K^+ \overline{K}^0} = -2 \, \langle K^- | ( \bar{s} c )_{S-P} | D^0 \rangle \langle K^+ | ( \bar{u} s )_{S+P} | 0 \rangle
\end{equation} 

%%%%

\begin{equation}
	\langle Q_6 \rangle_{tree; \pi^0 \pi^0} = - {2 \times} 2 \, \langle \pi^0 | ( \bar{u} c )_{S-P} | D^0 \rangle \langle \pi^0 | ( \bar{u} u )_{S+P} | 0 \rangle \label{eq:eq_Q6}\\
	%&& \langle Q_6 \rangle_{tree} = -2 \, \langle \pi^+ | ( \bar{u} c )_{S-P} | D^+ \rangle \langle \pi^0 | ( \bar{u} u )_{S+P} | 0 \rangle \nonumber
\end{equation}

\begin{equation}
	\langle Q_6 \rangle_{tree; \pi^+ \pi^0} = {\color{black} -} 2 \, \sqrt{2} \langle \pi^0 | ( \bar{u} c )_{S-P} | D^0 \rangle \langle \pi^0 | ( \bar{u} u )_{S+P} | 0 \rangle
\end{equation}
The extra factor of $ {2} $ in Eqs.~\eqref{eq:eq_Q2d}, \eqref{eq:eq_Q4}, \eqref{eq:eq_Q6} comes from identical particles in the final state.

%%%%%%%%%%%%%%%%%%%%%%%%%%%%%%%

For the form factors, we have ($ q = p_D - p_P $), $ x = d, s $, with kinematic constraint $ f^{D P}_+ (0) = f^{D P}_0 (0) $
%[likely, lattice references consider $ | D^+ \rangle = | c \bar{d} \rangle $, $ | D^0 \rangle = | c \bar{u} \rangle $, $ | \overline{K}^0 \rangle = | s \bar{d} \rangle $, $ | K^- \rangle = | s \bar{u} \rangle $, $ | \pi^- \rangle = | d \bar{u} \rangle $; I can't however decide on what lattice would take for $ | \pi^0 \rangle = \pm \frac{| d \bar{d} \rangle - | u \bar{u} \rangle}{\sqrt{2}} $?] I included the section of SU(4)xSU(4)
%[what if $ P = \pi^0 $?; in FLAG they say $ x = d, s $/not enough to conclude there is no $ \pi^0 $, and in fact there is]

\begin{equation}
	\langle P | ( \bar{x} c )_{V} | D \rangle = f^{D P}_+ (q^2) \left( {p_D}_\mu + {p_P}_\mu - \frac{M_D^2 - M_P^2}{q^2} q_\mu \right) + f^{D P}_0 (q^2) \frac{M_D^2 - M_P^2}{q^2} q_\mu
\end{equation}
%A part vanishes
and thus %[sign difference?, problem when comparing to Toni?/agrees w/ Schacht+]

\begin{equation}
	\langle P | ( \bar{x} c )_{S} | D \rangle = f^{D P}_0 (q^2) \frac{M_D^2 - M_P^2}{m_c - m_x}
\end{equation}

%\LVS{We assume that the values of $ f^{D \pi}_+, f^{D \pi}_0 $ given by Lattice calculations correspond to the flavours $ D^0, \pi^- $. [necessary to say?: these are isospin breaking corrections]}

For the decay constants (compared to App.~\ref{app:norm_sign_convs}, $ \sqrt{2} \, F = f $, and $f_\pi \neq f_K$ integrate further corrections)
%[likely, lattice references consider $ | \pi^+ \rangle = | u \bar{d} \rangle $ and $ | K^+ \rangle = | u \bar{s} \rangle $] I included the section of SU(4)xSU(4) %(the sign of the RH side flips when taking the complex conjugate; it is a global sign without practical effect) %[necessary, otherwise contracting and taking hermitian conjugate would not commute]

\begin{equation}
	\langle 0 | ( \bar{d} u )_A | \pi^+ (q) \rangle = i q_\mu f_{\pi^+} \,, \quad \langle 0 | ( \bar{s} u )_A | K^+ (q) \rangle = i q_\mu f_{K^+}
\end{equation}
and thus	

\begin{equation}
	\langle 0 | ( \bar{d} u )_P | \pi^+ (q) \rangle = -i \frac{M_\pi^2}{m_u + m_d} f_{\pi^+} \,, \quad \langle 0 | ( \bar{s} u )_P | K^+ (q) \rangle = -i \frac{M_K^2}{m_u + m_s} f_{K^+}
\end{equation}

%%%%%%%%%%%%%%%%%%%%%%%%%%%%%%%

Then:

\begin{equation}
	\langle Q_1^d \rangle_{tree; \pi^+ \pi^-} = \langle Q_4 \rangle_{tree; \pi^+ \pi^-} = i f_{\pi^+} f^{D \pi}_0 (M_\pi^2) (M_D^2 - M_\pi^2)
\end{equation}

\begin{equation}
	\langle Q_1^s \rangle_{tree; K^+ K^-} = \langle Q_4 \rangle_{tree; K^+ K^-} = i f_{K^+} f^{D K}_0 (M_K^2) (M_D^2 - M_K^2)
\end{equation}

\begin{eqnarray}
	&& \langle Q_6 \rangle_{tree; \pi^+ \pi^-} = -2 i f_{\pi^+} \frac{M_\pi^2}{m_u + m_d} f^{D \pi}_0 (M_\pi^2) \frac{M_D^2 - M_\pi^2}{m_c - m_d} \\
    && \qquad = -2 \frac{M_\pi^2}{m_u + m_d} \frac{1}{m_c - m_d} \langle Q_4 \rangle_{tree; \pi^+ \pi^-} \nonumber
\end{eqnarray}

\begin{eqnarray}
	&& \langle Q_6 \rangle_{tree; K^+ K^-} = -2 i f_{K^+} \frac{M_K^2}{m_u + m_s} f^{D K}_0 (M_K^2) \frac{M_D^2 - M_K^2}{m_c - m_s} \\
    && \qquad = -2 \frac{M_K^2}{m_u + m_s} \frac{1}{m_c - m_s} \langle Q_4 \rangle_{tree; K^+ K^-} \nonumber
\end{eqnarray}
The relative minus sign implies a cancellation among $ \langle Q_6 \rangle_{tree} $ and $ \langle Q_4 \rangle_{tree} $ (because their Wilson coefficients carry the same sign, see App.~\ref{app:num_inputs}).
Note that, at $ m_c \sim 1.3~\text{GeV} $:

\begin{equation}\label{eq:r_values}
	\frac{M_\pi^2}{m_u + m_d} \frac{1}{m_c - m_d} \simeq \frac{M_K^2}{m_u + m_s} \frac{1}{m_c - m_s} \simeq 2
\end{equation}
(not being then a sizable source of breaking of a potential symmetry relating pion and kaon channels).
%showing that $ m_c $ is comparable to $ v_{\langle \bar{q} q \rangle_0}/f_\pi^2 $, where $ -v_{\langle \bar{q} q \rangle_0} $ is the quark condensate

%%%%%%%%%%%%%%%%%%%%%%%%%%%%%%%

Finally:

\begin{equation}
	{\color{black} -} \langle Q_2^d \rangle_{tree; \pi^0 \pi^0} = \langle Q_4 \rangle_{tree; \pi^0 \pi^0} = {\color{black} +} {2 \times} \frac{1}{2} \langle Q_1^d \rangle_{tree; \pi^+ \pi^-} = {\color{black} +} {2 \times} \frac{1}{2} \langle Q_4 \rangle_{tree; \pi^+ \pi^-}
\end{equation}

\begin{equation}
	\langle Q_6 \rangle_{tree; \pi^0 \pi^0} = {\color{black} +} {2 \times} \frac{1}{2} \frac{m_c-m_d}{m_c-m_u} \frac{m_u+m_d}{2 \, m_u} \langle Q_6 \rangle_{tree; \pi^+ \pi^-}
\end{equation}

%[move to conventions only]
%\input{conventions.tex}

%%%%%%%%%%%%%%%%%%%%%%%%%%%%%%%

With the necessary elements dully provided, we then define, see Eq.~\eqref{eq:H_eff}:

\begin{eqnarray}
    && T^{CC}_{\pi^+ \pi^-} = -i G_F \, C_1 \, \lambda_d \, \langle Q_1^d \rangle_{tree; \pi^+ \pi^-} \\
    && T^{CC}_{\pi^0 \pi^0} = -i \frac{G_F}{\sqrt{2}} \, C_2 \, \lambda_d \, \langle Q_2^d \rangle_{tree; \pi^0 \pi^0} \\
    && T^{CC}_{K^+ K^-} = -i G_F \, C_1 \, \lambda_s \, \langle Q_1^s \rangle_{tree; K^+ K^-} \\
    && T^{CC}_{K^0 \overline{K}^0} = 0 \\
    && T^{P}_{\pi^+ \pi^-} = i G_F \, \lambda_b \left( C_4 \, \langle Q_4 \rangle_{tree; \pi^+ \pi^-} + C_6 \, \langle Q_6 \rangle_{tree; \pi^+ \pi^-} \right) \\
    && T^{P}_{\pi^0 \pi^0} = i \frac{G_F}{\sqrt{2}} \, \lambda_b \left( C_4 \, \langle Q_4 \rangle_{tree; \pi^0 \pi^0} + C_6 \, \langle Q_6 \rangle_{tree; \pi^0 \pi^0} \right) \\
    && T^{P}_{K^+ K^-} = i G_F \, \lambda_b \left( C_4 \, \langle Q_4 \rangle_{tree; K^+ K^-} + C_6 \, \langle Q_6 \rangle_{tree; K^+ K^-} \right) \\
    && T^{P}_{K^0 \overline{K}^0} = 0
\end{eqnarray}
where charged particles are to be taken as identical, see App.~\ref{app:isospin_decomposition}.

We consider the isospin limit, setting $ m_u, m_d \to \hat{m} $, see Tab.~\ref{tab:WCs}.

\section{\toni{OLD:} Isospin decomposition} %%%\label{app:isospin_decomposition}

%[\textbf{TODO:} discuss CPV in the charged decay mode (never discussed in the literature?) $D^+ \to \pi^+ \pi^0$; comments in personal notes]

The decomposition into states of definite isospin for pion pairs gives, employing the sign convention of Wigner \cite{Workman:2022ynf}:\footnote{Let $ \pi' $ be a triplet of $ SU(2) $

\begin{equation}
	\pi' =
	\begin{pmatrix}
	{\color{black} -} \pi_1 \\
	\pi_2 \\
	\pi_3 \\
	\end{pmatrix}
\end{equation}
which transforms as $ \pi' \to U \pi' $ in the spin-$1$ representation.
Alternatively, write the triplet as a $ 2 \times 2 $ traceless matrix

\begin{equation}
	\pi =
	\begin{pmatrix}
	{\color{black} +} \pi_2 / \sqrt{2} & \pi_1 \\
	\pi_3 & {\color{black} -} \pi_2 / \sqrt{2} \\
	\end{pmatrix}
\end{equation}
which transforms as $ \pi \to U \pi U^\dagger $ in the spin-$1/2$ representation, cf. Eq.~\eqref{eq:U4_U4_chiral}. Note the sign in front of $ \pi_1 $. The matrix $ U = 1 + i (\theta_1 T_1 + \theta_2 T_2 + \theta_3 T_3) $, with $ T_1, T_2, T_3 $ accordingly in the doublet or triplet representations.

We also identify the doublets $ \begin{pmatrix} K^+ \\ K^0 \\ \end{pmatrix} $ and $ \begin{pmatrix} \overline{D}^0 \\ D^- \\ \end{pmatrix} $, together with $ \begin{pmatrix} {\color{black} -} \overline{K}^0 \\ K^- \\ \end{pmatrix} = -i \sigma_2 \begin{pmatrix} K^+ \\ K^0 \\ \end{pmatrix}^\dagger $ and  $ \begin{pmatrix} {\color{black} -} D^+ \\ D^0 \\ \end{pmatrix} = -i \sigma_2 \begin{pmatrix} \overline{D}^0 \\ D^- \\ \end{pmatrix}^\dagger $.}

\begin{eqnarray}
	&& {\color{black} -} \langle \pi^+ \pi^- |_{id} = \sqrt{\frac{1}{3}} \langle 2\pi, I=2,M=0 | + \sqrt{\frac{2}{3}} \langle 2\pi, I=0,M=0 | \,, \\
	&& \langle \pi^0 \pi^0 | = \sqrt{\frac{2}{3}} \langle 2\pi, I=2,M=0 | - \sqrt{\frac{1}{3}} \langle 2\pi, I=0,M=0 |
\end{eqnarray}

\begin{eqnarray}
	&& \langle 2\pi, I=0,M=0 | = {\color{black} -} \sqrt{\frac{2}{3}} \langle \pi^+ \pi^- |_{id} - \sqrt{\frac{1}{3}} \langle \pi^0 \pi^0 | \,, \\
	&& \langle 2\pi, I=2,M=0 | = {\color{black} -} \sqrt{\frac{1}{3}} \langle \pi^+ \pi^- |_{id} + \sqrt{\frac{2}{3}} \langle \pi^0 \pi^0 |
\end{eqnarray}
The state $ \langle 2\pi, I=1,M=0 | = (\langle \pi^+_1 \pi^-_2 | - \langle \pi^-_1 \pi^+_2 |) / \sqrt{2} $ is not available by Bose-Einstein symmetry. We denote $ \langle \pi^+ \pi^- |_{id} = (\langle \pi^+_1 \pi^-_2 | + \langle \pi^-_1 \pi^+_2 |) / \sqrt{2} $, where the subscript ``id'' means that the $ \pi^\pm $ in $ \langle \pi^+ \pi^- |_{id} $ are to be taken as identical.

We will be denoting ($ T $ is the transition matrix):

\begin{eqnarray}
    && \langle 0 |T| D^0 \rangle = \langle 0 |T^{(1/2)}| D^0 \rangle = \mathcal{A}^\pi_0 + i \mathcal{B}^\pi_0 \\
    && \langle 2 |T^{(3/2)}| D^0 \rangle = \mathcal{A}^\pi_2 + i {\color{black} \mathcal{B}^\pi_2}
\end{eqnarray}
where $ \langle 2\pi, I=0,M=0 | \equiv \langle 0 | $ and $ \langle 2\pi, I=2,M=0 | \equiv \langle 2 | $, and $ \langle 2 |T| D^0 \rangle = \langle 2 |T^{(3/2)}| D^0 \rangle + \langle 2 |T^{(5/2)}| D^0 \rangle $. We will be neglecting $ \Delta I = 5/2 $ contributions.

Then

\begin{eqnarray}
	&& {\color{black} -} \langle \pi^+ \pi^- |_{id} T| D^0 \rangle = \sqrt{\frac{1}{3}} (\mathcal{A}^\pi_2 + i {\color{black} \mathcal{B}^\pi_2}) + \sqrt{\frac{2}{3}} ( \mathcal{A}^\pi_0 + i \mathcal{B}^\pi_0 ) \,, \\
	&& \langle \pi^0 \pi^0 |T| D^0 \rangle = \sqrt{\frac{2}{3}} (\mathcal{A}^\pi_2 + i {\color{black} \mathcal{B}^\pi_2}) - \sqrt{\frac{1}{3}} ( \mathcal{A}^\pi_0 + i \mathcal{B}^\pi_0 )
\end{eqnarray}

\begin{eqnarray}
	&& \langle 0 |T| D^0 \rangle = {\color{black} -} \sqrt{\frac{2}{3}} \langle \pi^+ \pi^- |_{id} T| D^0 \rangle - \sqrt{\frac{1}{3}} \langle \pi^0 \pi^0 |T| D^0 \rangle \,, \\
	&& \langle 2 |T| D^0 \rangle = {\color{black} -} \sqrt{\frac{1}{3}} \langle \pi^+ \pi^- |_{id} T| D^0 \rangle + \sqrt{\frac{2}{3}} \langle \pi^0 \pi^0 |T| D^0 \rangle
\end{eqnarray}

Also,

\begin{equation}
    \langle \pi^+ \pi^0 |_{id} T| D^+ \rangle = \langle \pi^+ \pi^0 |_{id} T^{(3/2)}| D^+ \rangle + \langle \pi^+ \pi^0 |_{id} T^{(5/2)}| D^+ \rangle
\end{equation}
with

\begin{equation}
	{\color{black} -} \langle \pi^+ \pi^0 |_{id} = {\color{black} -} \frac{1}{\sqrt{2}} ( \langle \pi^+_1 \pi^0_2 | + \langle \pi^0_1 \pi^+_2 | ) = \langle 2 \pi, 2, 1 |
\end{equation}

From Eckart-Wigner theorem, we have the following relation: %(the pre-factors are inverses of Clebsch-Gordan elements)

\begin{eqnarray}
	&& \sqrt{\frac{4}{3}} \langle 2, +1 | T^{(3/2)} | 1/2, + 1/2 \rangle = \sqrt{2} \langle 2,  0 | T^{(3/2)} | 1/2, - 1/2 \rangle %\\
	%&& - \sqrt{3}  \langle 2, +1 | T^{(5/2)} | 1/2, + 1/2 \rangle = \sqrt{2} \langle 2,  0 | T^{(5/2)} | 1/2, - 1/2 \rangle \nonumber
\end{eqnarray}
and thus

\begin{equation}
	{\color{black} -} \langle \pi^+ \pi^0 |_{id} T | 1/2, + 1/2 \rangle = {\color{black}{\color{black} +}} \langle \pi^+ \pi^0 |_{id} T | D^+ \rangle = \sqrt{\frac{3}{2}} (\mathcal{A}^\pi_2 + i {\color{black} \mathcal{B}^\pi_2})
\end{equation}
where we allow for a possibly non-vanishing $\mathcal{B}^\pi_2$ amplitude.
%[$\mathcal{B}^\pi_2$ depends on a single weak phase, the one of $\lambda_d$; suppose that $\mathcal{A}^\pi_2$ and $\mathcal{B}^\pi_2$ have different strong phases: then I could have CPV that would depend on the phase of $\lambda_d$ only, which is not rephasing-invariant?, so I can't have different strong phases?, true, they have the same leading $1/N_c$ expressions, when neglecting the contributions from penguin operators][if I have rescattering, I can possibly also have $\lambda_s$; note that two kaons do not form a state of total isospin-2; I could have an extra pair of pions (Bose-Einstein would not forbid having a total isospin-2)]
The dynamics of having contributions to $\mathcal{B}^\pi_2$ due to rescattering effects, making the process inelastic and introducing CP violation in this system, even in the isospin-conserving limit, will be discussed in a forthcoming publication \cite{PSVS_Ieq2:2023}.
%[relating the discussion about $G_4$ with $B_2^\pi$ is a good insight: we would indeed require some dynamics in $G_4$ (assuming the isospin-2 phase-shift does not flip value; I am overlooking $G_3$ (Leutwyler \cite{Leutwyler:2002hm} discusses P-wave, while here we are discussing S-wave)), which impacts the discussion of $D^+ \to \pi^+ \pi^0$; we are playing safe, however, because $A_2^\pi$ is being extracted from the branching ratio $D^+ \to \pi^+ \pi^0$, for which $B_2^\pi$ is irrelevant; see Donoghue, Gasser, Leutwyler on glueballs \cite{Donoghue:1990xh}]

For kaons:

\begin{eqnarray}
	&& \langle K^+_1 K^-_2 | = \frac{1}{\sqrt{2}} ( \langle 2K, 1, 0; 1/2_{\bar{s}} \; 1/2_s | + \langle 2K, 0, 0; 1/2_{\bar{s}} \; 1/2_s | ) \,, \\
%	&& \langle K^+ K^- |_{id} = \frac{1}{\sqrt{2}} ( \langle K^+ K^- | + \langle K^- K^+ | ) = \langle 2K, I = 0, M = 0 | + \langle 2K, I = 1, M = 0 | \,, \\ %NOT WELL NORMALIZED
	&& {\color{black} -} \langle K^0_1 \overline{K}^0_2 | = \frac{1}{\sqrt{2}} ( \langle 2K, 1, 0; 1/2_{\bar{s}} \; 1/2_s | - \langle 2K, 0, 0; 1/2_{\bar{s}} \; 1/2_s | )
%	&& \langle K^0 \bar{K}^0 |_{id} = \frac{1}{\sqrt{2}} ( \langle K^0 \bar{K}^0 | + \langle \bar{K}^0 K^0 | ) = - \langle 2K, I = 0, M = 0 | + \langle 2K, I = 1, M = 0 | \nonumber %NOT WELL NORMALIZED
\end{eqnarray}

\begin{eqnarray}
	&& \langle K^-_1 K^+_2 | = \frac{1}{\sqrt{2}} ( \langle 2K, 1, 0; 1/2_s \; 1/2_{\bar{s}} | - \langle 2K, 0, 0; 1/2_s \; 1/2_{\bar{s}} | ) \,, \\
	&& {\color{black} -} \langle \overline{K}^0_1 K^0_2 | = \frac{1}{\sqrt{2}} ( \langle 2K, 1, 0; 1/2_s \; 1/2_{\bar{s}} | + \langle 2K, 0, 0; 1/2_s \; 1/2_{\bar{s}} | )
\end{eqnarray}
which correspond to two possible additions of the kaon doublets.
\LVS{The first case (i.e., $1/2_{\bar{s}} \; 1/2_s$) would imply a negative sign in the off diagonal elements of Eq.~\eqref{eq:T00_expression}, while the second (i.e., $1/2_s \; 1/2_{\bar{s}}$) implies the positive sign displayed therein.} %[XCHECK which convention we are using; overall/relative sign?]
We recall the general rule for Clebsch-Gordan coefficients: %[manifests Bose symmetry]

\begin{equation}
	\langle j_1 j_2 m_1 m_2 | j_1 j_2 J M \rangle = (-1)^{J - j_1 - j_2} \langle j_2 j_1 m_2 m_1 | j_2 j_1 J M \rangle
\end{equation}
%%Then:

%\begin{eqnarray}
%	&& \langle K^+_1 K^-_2 | ( T | D^0 \rangle )_{\bar{s} s} = \frac{1}{\sqrt{2}} ( \langle 2K, 1, 0; 1/2_{\bar{s}} \; 1/2_s | ( T | D^0 \rangle )_{\bar{s} s} + \langle 2K, 0, 0; 1/2_{\bar{s}} \; 1/2_s | ( T | D^0 \rangle )_{\bar{s} s} ) \,, \nonumber\\
%	&& {\color{black} -} \langle K^0_1 \bar{K}^0_2 | ( T | D^0 \rangle )_{\bar{s} s} = \frac{1}{\sqrt{2}} ( \langle 2K, 1, 0; 1/2_{\bar{s}} \; 1/2_s | ( T | D^0 \rangle )_{\bar{s} s} - \langle 2K, 0, 0; 1/2_{\bar{s}} \; 1/2_s | ( T | D^0 \rangle )_{\bar{s} s} ) \nonumber
%\end{eqnarray}
%%\begin{eqnarray}
%%	&& \langle K^+_1 K^-_2 | ( T | D^0 \rangle )_{\bar{s} s} = \frac{1}{\sqrt{2}} ( \langle 2K, 1, 0; 1/2_s \; 1/2_{\bar{s}} | ( T | D^0 \rangle )_{s \bar{s}} - \langle 2K, 0, 0; 1/2_s \; 1/2_{\bar{s}} | ( T | D^0 \rangle )_{s \bar{s}} ) \,, \nonumber\\
%%	&& {\color{black} -} \langle K^0_1 \overline{K}^0_2 | ( T | D^0 \rangle )_{\bar{s} s} = \frac{1}{\sqrt{2}} ( \langle 2K, 1, 0; 1/2_s \; 1/2_{\bar{s}} | ( T | D^0 \rangle )_{s \bar{s}} + \langle 2K, 0, 0; 1/2_s \; 1/2_{\bar{s}} | ( T | D^0 \rangle )_{s \bar{s}} ) \nonumber
%%\end{eqnarray}

%\begin{eqnarray}
%	&& \langle K^-_1 K^+_2 | ( T | D^0 \rangle )_{s \bar{s}} = \frac{1}{\sqrt{2}} ( \langle 2K, 1, 0; 1/2_{\bar{s}} \; 1/2_s | ( T | D^0 \rangle )_{\bar{s} s} + \langle 2K, 0, 0; 1/2_{\bar{s}} \; 1/2_s | ( T | D^0 \rangle )_{\bar{s} s} ) \,, \nonumber\\
%	&& {\color{black} -} \langle \bar{K}^0_1 K^0_2 | ( T | D^0 \rangle )_{s \bar{s}} = \frac{1}{\sqrt{2}} ( \langle 2K, 1, 0; 1/2_{\bar{s}} \; 1/2_s | ( T | D^0 \rangle )_{\bar{s} s} - \langle 2K, 0, 0; 1/2_{\bar{s}} \; 1/2_s | ( T | D^0 \rangle )_{\bar{s} s} ) \nonumber
%\end{eqnarray}
%%\begin{eqnarray}
%%	&& \langle K^-_1 K^+_2 | ( T | D^0 \rangle )_{s \bar{s}} = \frac{1}{\sqrt{2}} ( \langle 2K, 1, 0; 1/2_s \; 1/2_{\bar{s}} | ( T | D^0 \rangle )_{s \bar{s}} - \langle 2K, 0, 0; 1/2_s \; 1/2_{\bar{s}} | ( T | D^0 \rangle )_{s \bar{s}} ) \,, \nonumber\\
%%	&& {\color{black} -} \langle \overline{K}^0_1 K^0_2 | ( T | D^0 \rangle )_{s \bar{s}} = \frac{1}{\sqrt{2}} ( \langle 2K, 1, 0; 1/2_s \; 1/2_{\bar{s}} | ( T | D^0 \rangle )_{s \bar{s}} + \langle 2K, 0, 0; 1/2_s \; 1/2_{\bar{s}} | ( T | D^0 \rangle )_{s \bar{s}} ) \nonumber
%%\end{eqnarray}

\noindent
We now define the symmetric combinations: %%(we now drop the subscript of $T | D^0 \rangle$)

%\begin{eqnarray}
%	&& \frac{\langle K^+_1 K^-_2 | T | D^0 \rangle + \langle K^-_1 K^+_2 | T | D^0 \rangle}{\sqrt{2}} = \langle 2K, 1, 0; 1/2_{\bar{s}} \; 1/2_s | T | D^0 \rangle + \langle 2K, 0, 0; 1/2_{\bar{s}} \; 1/2_s | T | D^0 \rangle \,, \nonumber\\
%	&& {\color{black} -} \frac{\langle K^0_1 \bar{K}^0_2 | T | D^0 \rangle + \langle \bar{K}^0_1 K^0_2 | T | D^0 \rangle}{\sqrt{2}} = \langle 2K, 1, 0; 1/2_{\bar{s}} \; 1/2_s | T | D^0 \rangle - \langle 2K, 0, 0; 1/2_{\bar{s}} \; 1/2_s | T | D^0 \rangle \nonumber
%\end{eqnarray}
\begin{eqnarray}
	&& \frac{\langle K^+_1 K^-_2 | T | D^0 \rangle + \langle K^-_1 K^+_2 | T | D^0 \rangle}{\sqrt{2}} \\
    && \qquad = \langle 2K, 1, 0; 1/2_s \; 1/2_{\bar{s}} | T | D^0 \rangle - \langle 2K, 0, 0; 1/2_s \; 1/2_{\bar{s}} | T | D^0 \rangle \,,  \nonumber\\
	&& {\color{black} -} \frac{\langle K^0_1 \overline{K}^0_2 | T | D^0 \rangle + \langle \overline{K}^0_1 K^0_2 | T | D^0 \rangle}{\sqrt{2}} \\
    && \qquad = \langle 2K, 1, 0; 1/2_s \; 1/2_{\bar{s}} | T | D^0 \rangle + \langle 2K, 0, 0; 1/2_s \; 1/2_{\bar{s}} | T | D^0 \rangle \nonumber
\end{eqnarray}

Introduce now:

%\begin{eqnarray}
%    && \langle 2K, 0, 0; 1/2_{\bar{s}} \; 1/2_s | T | D^0 \rangle = \langle 2K, 0, 0; 1/2_{\bar{s}} \; 1/2_s | T^{(1/2)} | D^0 \rangle = \mathcal{A}^K_0 + i \mathcal{B}^K_0 \\
%    && \langle 2K, 1, 0 | T | D^0 \rangle = \langle 2K, 1, 0 | T^{(1/2)} | D^0 \rangle + \langle 2K, 1, 0 | T^{(3/2)} | D^0 \rangle \\
%    && \langle 2K, 1, 0; 1/2_{\bar{s}} \; 1/2_s | T^{(1/2)} | D^0 \rangle = \mathcal{A}^K_{11} + i \mathcal{B}^K_{11} \\
%    && \langle 2K, 1, 0; 1/2_{\bar{s}} \; 1/2_s | T^{(3/2)} | D^0 \rangle = \mathcal{A}^K_{13} + i {\color{black} \mathcal{B}^K_{13}}
%\end{eqnarray}
\begin{eqnarray}
    && \langle 2K, 0, 0; 1/2_s \; 1/2_{\bar{s}} | T | D^0 \rangle = \langle 2K, 0, 0; 1/2_s \; 1/2_{\bar{s}} | T^{(1/2)} | D^0 \rangle = \mathcal{A}^K_0 + i \mathcal{B}^K_0 \\
    && \langle 2K, 1, 0 | T | D^0 \rangle = \langle 2K, 1, 0 | T^{(1/2)} | D^0 \rangle + \langle 2K, 1, 0 | T^{(3/2)} | D^0 \rangle \\
    && \langle 2K, 1, 0; 1/2_s \; 1/2_{\bar{s}} | T^{(1/2)} | D^0 \rangle = \mathcal{A}^K_{11} + i \mathcal{B}^K_{11} \\
    && \langle 2K, 1, 0; 1/2_s \; 1/2_{\bar{s}} | T^{(3/2)} | D^0 \rangle = \mathcal{A}^K_{13} + i {\color{black} \mathcal{B}^K_{13}}
\end{eqnarray}
With that, we write:

%\begin{eqnarray}
%	&& \langle K^+ K^- |_{id} T| D^0 \rangle = (\mathcal{A}^K_0 + i \mathcal{B}^K_0) + (\mathcal{A}^K_{11} + i \mathcal{B}^K_{11}) + (\mathcal{A}^K_{13} + i {\color{black} \mathcal{B}^K_{13}}) \\
%	&& {\color{black} -} \langle K^0 \bar{K}^0 |_{id} T| D^0 \rangle = - (\mathcal{A}^K_0 + i \mathcal{B}^K_0) + (\mathcal{A}^K_{11} + i \mathcal{B}^K_{11}) + (\mathcal{A}^K_{13} + i {\color{black} \mathcal{B}^K_{13}})
%\end{eqnarray}
\begin{eqnarray}
	&& \langle K^+ K^- |_{id} T| D^0 \rangle = - (\mathcal{A}^K_0 + i \mathcal{B}^K_0) + (\mathcal{A}^K_{11} + i \mathcal{B}^K_{11}) + (\mathcal{A}^K_{13} + i {\color{black} \mathcal{B}^K_{13}}) \\
	&& {\color{black} -} \langle K^0 \overline{K}^0 |_{id} T| D^0 \rangle = (\mathcal{A}^K_0 + i \mathcal{B}^K_0) + (\mathcal{A}^K_{11} + i \mathcal{B}^K_{11}) + (\mathcal{A}^K_{13} + i {\color{black} \mathcal{B}^K_{13}})
\end{eqnarray}

From Eckart-Wigner:

\begin{eqnarray}
	&& - \sqrt{4} \langle 1, +1 | T^{(3/2)} | 1/2, + 1/2 \rangle = \sqrt{2} \langle 1,  0 | T^{(3/2)} | 1/2, - 1/2 \rangle \\
	&& \langle 1, +1 | T^{(1/2)} | 1/2, + 1/2 \rangle = \sqrt{2} \langle 1,  0 | T^{(1/2)} | 1/2, - 1/2 \rangle %=\sqrt{2} \langle 0,  0 | T^{(1/2)} | 1/2, - 1/2 \rangle, NOT FROM Wigner-Eckart
\end{eqnarray}
Since:

\begin{equation}
	{\color{black} -} \langle K^+_1 \overline{K}^0_2 | = \langle 2 K, 1, 1; 1/2_{\bar{s}} \; 1/2_s |
%	{\color{red} \langle K^+ \bar{K}^0 |_{id} = \frac{1}{\sqrt{2}} ( \langle K^+ \bar{K}^0 | + \langle \bar{K}^0 K^+ | ) = \sqrt{2} \langle 2 K, 1, 1 | } %NOT WELL NORMALIZED
\end{equation}
and thus

\begin{equation}
	\langle K^+ \overline{K}^0 |_{id} T | D^+ \rangle = 2 ( \mathcal{A}^K_{11} + i \mathcal{B}^K_{11} ) - (\mathcal{A}^K_{13} + i {\color{black} \mathcal{B}^K_{13}})
\end{equation}

%%%%%%%%%%%%%%%%%%%%%%%%%%%%%%%

\subsection{Physical kaons}\label{app:physical_kaons}

We have the following reciprocal states \cite{Branco:1999fs}:

\begin{equation}
	\langle K_L | = \frac{1}{2 p_K} \langle K^0 | + \frac{1}{2 q_K} \langle \overline{K}^0 | \,, \quad \langle K_S | = \frac{1}{2 p_K} \langle K^0 | - \frac{1}{2 q_K} \langle \overline{K}^0 |
\end{equation}
To leading order in weak interactions:

\begin{eqnarray}
	\langle K^+ \overline{K}^0 | T | D^+ \rangle = \langle K^+ | \otimes \left( \langle K_L | - \langle K_S | \right) q_K T | D^+ \rangle \\
	0 \sim \langle K^+ K^0 | T | D^+ \rangle = \langle K^+ | \otimes \left( \langle K_L | + \langle K_S | \right) p_K T | D^+ \rangle
\end{eqnarray}
then

\begin{eqnarray}
	&& \langle K^+ K_L | T | D^+ \rangle \simeq \frac{\langle K^+ \overline{K}^0 | T | D^+ \rangle}{2 q_K} \,,\; \langle K^- K_L | T | D^- \rangle \simeq \frac{\langle K^- K^0 | T | D^- \rangle}{2 p_K} \\
	&& \langle K^+ K_S | T | D^+ \rangle \simeq -\frac{\langle K^+ \overline{K}^0 | T | D^+ \rangle}{2 q_K} \,,\; \langle K^- K_S | T | D^- \rangle \simeq \frac{\langle K^- K^0 | T | D^- \rangle}{2 p_K}
\end{eqnarray}
Similarly

\begin{eqnarray}
	\langle K^0 \overline{K}^0 | T | D^0 \rangle = \left( \langle K_L | + \langle K_S | \right) p_K \otimes \left( \langle K_L | - \langle K_S | \right) q_K T | D^0 \rangle \\
	\langle \overline{K}^0 K^0 | T | D^0 \rangle = \left( \langle K_L | - \langle K_S | \right) q_K \otimes \left( \langle K_L | + \langle K_S | \right) p_K T | D^0 \rangle \\
	0 \sim \langle K^0 K^0 | T | D^0 \rangle = \left( \langle K_L | + \langle K_S | \right) p_K \otimes \left( \langle K_L | + \langle K_S | \right) p_K T | D^0 \rangle \\
	0 \sim \langle \overline{K}^0 \overline{K}^0 | T | D^0 \rangle = \left( \langle K_L | - \langle K_S | \right) q_K \otimes \left( \langle K_L | - \langle K_S | \right) q_K T | D^0 \rangle
\end{eqnarray}
then

\begin{equation}
	\frac{\sqrt{2}}{2 p_K q_K} \langle K^0 \overline{K}^0 |_{id} T | D^0 \rangle = \left( \langle K_L K_L | - \langle K_S K_S | \right) T | D^0 \rangle \,,\; 0 \sim \left( \langle K_L K_L | + \langle K_S K_S | \right) T | D^0 \rangle
\end{equation}

\begin{equation}
	\left( \frac{\langle K_S K_L | + \langle K_L K_S |}{\sqrt{2}} \right) T | D^0 \rangle \sim 0 \sim \left( \frac{\langle K_S K_L | + \langle K_L K_S |}{\sqrt{2}} \right) T | \overline{D}^0 \rangle
\end{equation}
and

\begin{eqnarray}
	&& \langle K_L K_L | T | D^0 \rangle \simeq \frac{\sqrt{2}}{4 p_K q_K} \langle K^0 \overline{K}^0 |_{id} T | D^0 \rangle \simeq -\langle K_S K_S | T | D^0 \rangle \\
	&& \langle K_L K_L | T | \overline{D}^0 \rangle \simeq \frac{\sqrt{2}}{4 p_K q_K} \langle K^0 \overline{K}^0 |_{id} T | \overline{D}^0 \rangle \simeq -\langle K_S K_S | T | \overline{D}^0 \rangle
\end{eqnarray}
where we make use of the symmetrized combination %[\textbf{note the normalization}: agrees with the previous section]

\begin{equation}
	\langle K^0 \overline{K}^0 |_{id} = \frac{\langle K^0 \overline{K}^0 | + \langle \overline{K}^0 K^0 |}{\sqrt{2}}
\end{equation}
already introduced above.
We have that: $ | p_K |^2 = (1 + \delta) / 2 $, $ | q_K |^2 = (1 - \delta) / 2 $; $ | \delta | \ll 1 $ and is neglected.

%%%%%%%%%%%%%%%%%%%%%%%%%%%%%%%

\section{Simplified expressions}\label{app:simplified_expressions}

For illustrative purposes only,
we give expressions valid in the limits $ M_\pi^2 / M_D^2 $, $ M_K^2 / M_D^2 \to 0^+ $ ($ m_u / m_c $, $ m_d / m_c $, $ m_s / m_c \to 0^+ $), $ f_K / f_\pi $, $ F^{D K}_0 (0) / F^{D \pi}_0 (0) \to 1 $ (both ratios being in reality $\simeq 1.2$), and $ \text{Re} \{ \lambda_b \} \to 0 $ (since $ | \lambda_b | $ is rephasing invariant, and much smaller than $ | \lambda_d |, | \lambda_s | $):

%%%%%%%%%%%%%%%%%%%%%%%%

\begin{equation}
	\mathcal{A}^\pi_0 \simeq - \frac{f_\pi G_F M_D^2 F^{D \pi}_0 (0)}{\sqrt{6}} \left[ (2 C_1 - C_2) \, \Omega^{(0)}_{1 1} \, \text{Re} \{ \lambda_d \} + \frac{\sqrt{3}}{\sqrt{2}} \, C_1 \, \Omega^{(0)}_{1 2} \, \text{Re} \{ \lambda_s \} \right]
\end{equation}

\begin{eqnarray}
	&& \mathcal{B}^\pi_0 \simeq - \frac{f_\pi G_F M_D^2 F^{D \pi}_0 (0)}{\sqrt{6}} \left[ (2 C_1 - C_2) \, \Omega^{(0)}_{1 1} \, \text{Im} \{ \lambda_d \} + \frac{\sqrt{3}}{\sqrt{2}} \, C_1 \, \Omega^{(0)}_{1 2} \, \text{Im} \{ \lambda_s \} \right. \\
    && \qquad\qquad\quad \left. - \frac{\sqrt{3}}{\sqrt{2}} \, ( C_4 - C_6 \, \delta^\pi_6 ) \, (\Omega^{(0)}_{1 2} + \sqrt{6} \, \Omega^{(0)}_{1 1}) \, \text{Im} \{ \lambda_b \} \right] \nonumber
\end{eqnarray}

%%%%%%%%%%%%%%%%%%%%%%%%

\begin{equation}
	\mathcal{A}^K_0 \simeq - \frac{f_K G_F M_D^2 F^{D K}_0 (0)}{\sqrt{6}} \left[ (2 C_1 - C_2) \, \Omega^{(0)}_{2 1} \, \text{Re} \{ \lambda_d \} + \frac{\sqrt{3}}{\sqrt{2}} \, C_1 \, \Omega^{(0)}_{2 2} \, \text{Re} \{ \lambda_s \} \right]
\end{equation}

\begin{eqnarray}
	&& \mathcal{B}^K_0 \simeq - \frac{f_K G_F M_D^2 F^{D K}_0 (0)}{\sqrt{6}} \left[ (2 C_1 - C_2) \, \Omega^{(0)}_{2 1} \, \text{Im} \{ \lambda_d \} + \frac{\sqrt{3}}{\sqrt{2}} \, C_1 \, \Omega^{(0)}_{2 2} \, \text{Im} \{ \lambda_s \} \right. \\
    && \qquad\qquad\quad \left. - \frac{\sqrt{3}}{\sqrt{2}} \, ( C_4 - C_6 \, \delta^K_6 ) \, (\Omega^{(0)}_{2 2} + \sqrt{6} \, \Omega^{(0)}_{2 1}) \, \text{Im} \{ \lambda_b \} \right] \nonumber
\end{eqnarray}

%%%%%%%%%%%%%%%%%%%%%%%%

\begin{equation}
	\mathcal{A}^\pi_2 \simeq - \frac{f_\pi G_F M_D^2 F^{D \pi}_0 (0)}{\sqrt{3}} \, (C_1 + C_2) \, |\Omega^{(2)}| e^{i \phi_2} \, \text{Re} \{ \lambda_d \}
\end{equation}

\begin{equation}
	\mathcal{B}^\pi_2 \simeq - \frac{f_\pi G_F M_D^2 F^{D \pi}_0 (0)}{\sqrt{3}} \, (C_1 + C_2) \, |\Omega^{(2)}| e^{i \phi_2} \, \text{Im} \{ \lambda_d \}
\end{equation}

%%%%%%%%%%%%%%%%%%%%%%%%

\begin{equation}
	\mathcal{A}^K_{11} \simeq \frac{f_K G_F M_D^2 F^{D K}_0 (0)}{2} \, C_1 \, |\Omega^{(1)}| e^{i \phi_1} \, \text{Re} \{ \lambda_s \}
\end{equation}

\begin{equation}
	\mathcal{B}^K_{11} \simeq \frac{f_K G_F M_D^2 F^{D K}_0 (0)}{2} \, |\Omega^{(1)}| e^{i \phi_1} \left[ C_1  \, \text{Im} \{ \lambda_s \} - ( C_4 - C_6 \, \delta^K_6 )  \, \text{Im} \{ \lambda_b \} \right]
\end{equation}

%where $R_{\pi, K}$ are the expressions seen in Eq.~\eqref{eq:r_values}: $ R_\pi \equiv \frac{2 M_\pi^2}{2 \, \hat{m} \, (m_c - \hat{m})} $, $ R_K \equiv \frac{2 M_K^2}{(m_s + \hat{m}) \, (m_c - m_s)} $.

%%%%%%%%%%%%%%%%%%%%%%%%

%\begin{equation}
%	\tan \arg \mathcal{A}^\pi_0 \simeq \frac{\sqrt{2} \, (2 C_1 - C_2) \, \text{Im} [ \Omega_{1 1} ] \, \text{Re} \{ \lambda_d \} + \sqrt{3} \, C_1 \, \text{Im} [ \Omega_{1 2} ] \, \text{Re} \{ \lambda_s \}}{\sqrt{2} \, (2 C_1 - C_2) \, \text{Re} [ \Omega_{1 1} ] \, \text{Re} \{ \lambda_d \} + \sqrt{3} \, C_1 \, \text{Re} [ \Omega_{1 2} ] \, \text{Re} \{ \lambda_s \}}
%\end{equation}

%\begin{eqnarray}
%	&& \qquad\qquad\quad \tan \arg \mathcal{B}^\pi_0 \simeq \\
%    && \frac{\sqrt{2} \, (2 C_1 - C_2) \, \text{Im} [ \Omega_{1 1} ] \, \text{Im} \{ \lambda_d \} + \sqrt{3} \, C_1 \, \text{Im} [ \Omega_{1 2} ] \, \text{Im} \{ \lambda_s \} - \sqrt{3} \, C_4 \, (\sqrt{6} \text{Im} [ \Omega_{1 1} ] + \text{Im} [ \Omega_{1 2} ]) \, \text{Im} \{ \lambda_b \}}{\sqrt{2} \, (2 C_1 - C_2) \, \text{Re} [ \Omega_{1 1} ] \, \text{Im} \{ \lambda_d \} + \sqrt{3} \, C_1 \, \text{Re} [ \Omega_{1 2} ] \, \text{Im} \{ \lambda_s \} - \sqrt{3} \, C_4 \, (\sqrt{6} \text{Re} [ \Omega_{1 1} ] + \text{Re} [ \Omega_{1 2} ]) \, \text{Im} \{ \lambda_b \}} \nonumber
%\end{eqnarray}

%%%%%%%%%%%%%%%%%%%%%%%%

%\begin{equation}
%	\tan \arg \mathcal{A}^K_0 \simeq \frac{\sqrt{2} \, (2 C_1 - C_2) \, \text{Im} [ \Omega_{2 1} ] \, \text{Re} \{ \lambda_d \} + \sqrt{3} \, C_1 \, \text{Im} [ \Omega_{2 2} ] \, \text{Re} \{ \lambda_s \}}{\sqrt{2} \, (2 C_1 - C_2) \, \text{Re} [ \Omega_{2 1} ] \, \text{Re} \{ \lambda_d \} + \sqrt{3} \, C_1 \, \text{Re} [ \Omega_{2 2} ] \, \text{Re} \{ \lambda_s \}}
%\end{equation}

%\begin{eqnarray}
%	&& \qquad\qquad\quad \tan \arg \mathcal{B}^K_0 \simeq \\
%    && \frac{\sqrt{2} \, (2 C_1 - C_2) \, \text{Im} [ \Omega_{2 1} ] \, \text{Im} \{ \lambda_d \} + \sqrt{3} \, C_1 \, \text{Im} [ \Omega_{2 2} ] \, \text{Im} \{ \lambda_s \} - \sqrt{3} \, C_4 \, (\sqrt{6} \text{Im} [ \Omega_{2 1} ] + \text{Im} [ \Omega_{2 2} ]) \, \text{Im} \{ \lambda_b \}}{\sqrt{2} \, (2 C_1 - C_2) \, \text{Re} [ \Omega_{2 1} ] \, \text{Im} \{ \lambda_d \} + \sqrt{3} \, C_1 \, \text{Re} [ \Omega_{2 2} ] \, \text{Im} \{ \lambda_s \} - \sqrt{3} \, C_4 \, (\sqrt{6} \text{Re} [ \Omega_{2 1} ] + \text{Re} [ \Omega_{2 2} ]) \, \text{Im} \{ \lambda_b \}} \nonumber
%\end{eqnarray}

%%%%%%%%%%%%%%%%%%%%%%%%

%\noindent
%where
%$\mathcal{Y} = \mathcal{A}, \mathcal{B}$ with respectively $\text{X} = \text{Re}, \text{Im}$;
%$ P $ stands for $ \pi $ or $ K $.

%\input{numerical_results.tex}
